# Supplementary material for: HiveNAS: Neural Architecture Search using Artificial Bee Colony Optimization
Source: arXiv:2211.10250 source file (2023-06-15)
Supplement: Supplementary file 1 [file AppendixA.tex]

\section{Top-Performing Candidates}

\begin{figure}[!htbp]
\centering
\includegraphics[width=0.95\textwidth]{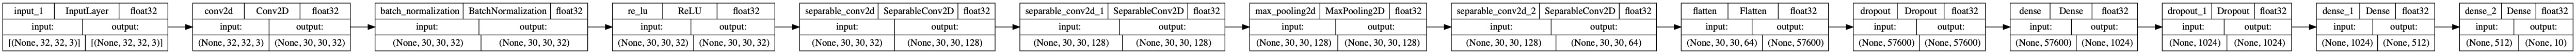}
\caption{Baseline model architecture}
\end{figure}

\begin{figure}[!htbp]
\centering
\includegraphics[width=0.95\textwidth]{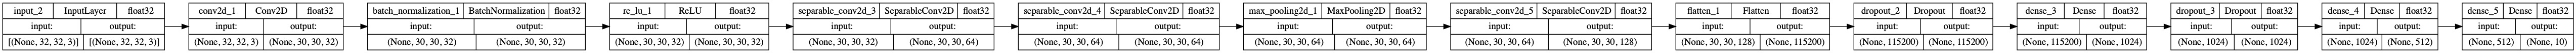}
\caption{HiveNAS+Aug model architecture}
\end{figure}

\begin{figure}[!htbp]
\centering
\includegraphics[width=0.95\textwidth]{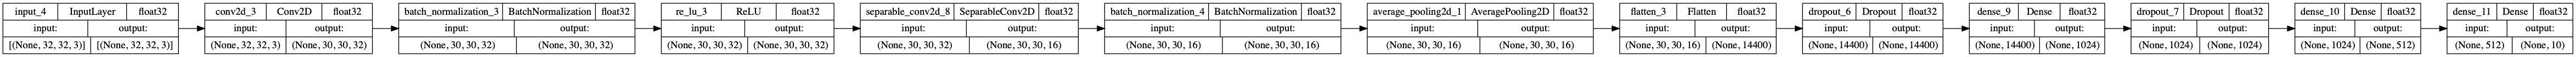}
\caption{HiveNAS+Cutout model architecture}
\end{figure}

\begin{figure}[!htbp]
\centering
\includegraphics[width=0.95\textwidth]{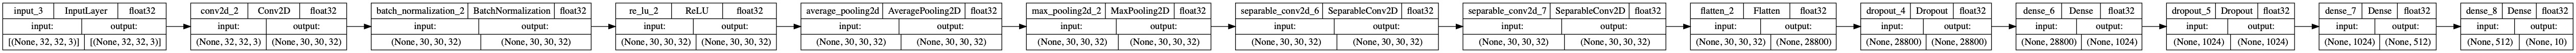}
\caption{HiveNAS+ResNet model architecture}
\end{figure}

% \begin{figure}[!htbp]
% \centering
% \includegraphics[width=0.95\textwidth]{figures/HiveNAS+ACT_arch.jpg}
% \caption{HiveNAS+ACT model architecture}
% \end{figure}
